# Supplementary material for: Analytical amplitudes from numerical solutions of the scattering equations
Source: arXiv:1910.11355 ancillary file (2019-12-17)
Supplement: Supplementary file 1 [file 4pt.pdf]

$$\frac{-12(13)[13]}{(12)/(23)/(12)[23]}$$

$$\frac{1}{(\mathbf{12})[\mathbf{12}]} +$$

$$\frac{1}{(\mathbf{23})[\mathbf{23}]}$$
