# Supplementary material for: Analytical amplitudes from numerical solutions of the scattering equations
Source: arXiv:1910.11355 ancillary file (2019-12-17)
Supplement: Supplementary file 2 [file ppppp.pdf]

$$\frac{1i[12]\langle 13\rangle\langle 25\rangle[35]^2}{\langle 12\rangle^2\langle 34\rangle\langle 45\rangle} +$$

$$\frac{1i[14][24][35]}{\langle 12\rangle\langle 35\rangle} +$$

$$(12345 \rightarrow 23451) +$$

$$(12345 \rightarrow 34512) +$$

$$(12345 \rightarrow 45123) +$$

$$(12345 \rightarrow 51234) +$$

$$\frac{2i[15][23]\langle 4|1+2|4\rangle}{\langle 12\rangle\langle 34\rangle\langle 45\rangle} +$$

$$\frac{2i[12][45]\langle 3|1+5|3\rangle}{\langle 15\rangle\langle 23\rangle\langle 34\rangle} +$$

$$\frac{2i[12][15][34]}{\langle 23\rangle\langle 45\rangle}$$

$$\frac{-4i(12)^5[12]^2(13)^2[13](24)(34)(35)^2(45)^2 \dots \langle 135 \text{ terms} \rangle \dots -1i[12](13)^4(14)[23](24)^4[24](25)^3(35)}{(12)^2(13)(14)(15)^2(23)^2(24)(25)(34)^2(35)(45)^2}$$
