# Supplementary material for: Analytical amplitudes from numerical solutions of the scattering equations
Source: arXiv:1910.11355 ancillary file (2019-12-17)
Supplement: Supplementary file 3 [file pppmmm_from_bcfw.pdf]

$$\frac{-1i[23]^7\langle 34\rangle\langle 56\rangle^7[56]}{\langle 15\rangle\langle 16\rangle[24][34]\langle 1|2+4|3\rangle\langle 1|2+3|4\rangle\langle 5|1+6|2\rangle\langle 6|1+5|2\rangle s_{234}} +$$

$$\frac{[24]\langle 4|1+2|3\rangle^7(-1i\langle 12\rangle[12]\langle 13\rangle[35]\langle 45\rangle \dots \langle 6 \text{ terms} \rangle \dots + 1i\langle 14\rangle[24]\langle 25\rangle\langle 34\rangle[35])}{\langle 12\rangle^2\langle 24\rangle[35][36][56]\langle 1|2+4|3\rangle\langle 1|2+4|5\rangle\langle 1|2+4|6\rangle\langle 4|1+2|5\rangle\langle 4|1+2|6\rangle s_{124}} +$$

$$\frac{[12]^6\langle 14\rangle\langle 56\rangle^7(-1i\langle 12\rangle[12][23]\langle 35\rangle[45] \dots \langle 6 \text{ terms} \rangle \dots - 1i[23]\langle 24\rangle[24]\langle 35\rangle[45])}{[14]\langle 35\rangle\langle 36\rangle\langle 3|1+4|2\rangle\langle 3|1+2|4\rangle\langle 5|1+4|2\rangle\langle 5|1+2|4\rangle\langle 6|1+4|2\rangle\langle 6|1+2|4\rangle s_{124}} +$$

$$\frac{-1i[34]\langle 56\rangle\langle 4|1+3|2\rangle^7}{\langle 13\rangle\langle 14\rangle[25][26]\langle 34\rangle[56]\langle 1|2+6|5\rangle\langle 1|2+5|6\rangle\langle 3|1+4|2\rangle s_{134}} +$$

$$(123456 \rightarrow 123546)+$$

$$(123456 \rightarrow 123654)+$$

$$\frac{[23]s_{123}^7(1i\langle 12\rangle\langle 13\rangle[14][25]\langle 45\rangle \dots \langle 6 \text{ terms} \rangle \dots - 1i\langle 13\rangle[23]\langle 25\rangle\langle 34\rangle[45])}{\langle 12\rangle^2\langle 23\rangle[45][46][56]\langle 1|2+3|4\rangle\langle 1|2+3|5\rangle\langle 1|2+3|6\rangle\langle 3|1+2|4\rangle\langle 3|1+2|5\rangle\langle 3|1+2|6\rangle}$$

$$\begin{aligned}
& \frac{-1i[23]^7\langle 34\rangle\langle 56\rangle^7[56]}{\langle 15\rangle\langle 16\rangle[24][34]\langle 1|2+4|3\rangle\langle 1|2+3|4\rangle\langle 5|1+6|2\rangle\langle 6|1+5|2\rangle s_{234}} + \\
& \frac{-1i[23]^7\langle 35\rangle\langle 46\rangle^7[46]}{\langle 14\rangle\langle 16\rangle[25][35]\langle 1|2+5|3\rangle\langle 1|2+3|5\rangle\langle 4|1+6|2\rangle\langle 6|1+4|2\rangle s_{235}} + \\
& \frac{-1i[23]^7\langle 36\rangle\langle 45\rangle^7[45]}{\langle 14\rangle\langle 15\rangle[26][36]\langle 1|2+6|3\rangle\langle 1|2+3|6\rangle\langle 4|1+5|2\rangle\langle 5|1+4|2\rangle s_{145}} + \\
& \frac{-1i[34]\langle 56\rangle\langle 4|1+3|2\rangle^7}{\langle 13\rangle\langle 14\rangle[25][26]\langle 34\rangle\langle 56\rangle\langle 1|2+6|5\rangle\langle 1|2+5|6\rangle\langle 3|1+4|2\rangle s_{134}} + \\
& \frac{-1i[35]\langle 46\rangle\langle 5|1+3|2\rangle^7}{\langle 13\rangle\langle 15\rangle[24][26]\langle 35\rangle\langle 46\rangle\langle 1|2+6|4\rangle\langle 1|2+4|6\rangle\langle 3|1+5|2\rangle s_{135}} + \\
& \frac{-1i[36]\langle 45\rangle\langle 6|1+3|2\rangle^7}{\langle 13\rangle\langle 16\rangle[24][25]\langle 36\rangle\langle 45\rangle\langle 1|2+5|4\rangle\langle 1|2+4|5\rangle\langle 3|1+6|2\rangle s_{245}} + \\
& \frac{[24]\langle 4|1+2|3\rangle^7(-1i\langle 12\rangle[12]\langle 13\rangle[35]\langle 45\rangle \dots \langle 6 \text{ terms} \rangle \dots +1i\langle 14\rangle[24]\langle 25\rangle\langle 34\rangle[35])}{\langle 12\rangle^2[24][35][36][56]\langle 1|2+4|3\rangle\langle 1|2+4|5\rangle\langle 1|2+4|6\rangle\langle 4|1+2|5\rangle\langle 4|1+2|6\rangle s_{124}} + \\
& \frac{[12]^6\langle 14\rangle\langle 56\rangle^7(-1i\langle 12\rangle[12][23]\langle 35\rangle\langle 45\rangle \dots \langle 6 \text{ terms} \rangle \dots -1i[23]\langle 24\rangle[24]\langle 35\rangle\langle 45\rangle)}{[14]\langle 35\rangle\langle 36\rangle\langle 3|1+4|2\rangle\langle 3|1+2|4\rangle\langle 5|1+4|2\rangle\langle 5|1+2|4\rangle\langle 6|1+4|2\rangle\langle 6|1+2|4\rangle s_{124}} + \\
& \frac{[25]\langle 5|1+2|3\rangle^7(1i\langle 12\rangle[12]\langle 13\rangle[34]\langle 45\rangle \dots \langle 6 \text{ terms} \rangle \dots -1i\langle 15\rangle[24]\langle 25\rangle\langle 34\rangle[35])}{\langle 12\rangle^2\langle 25\rangle[34][36][46]\langle 1|2+5|3\rangle\langle 1|2+5|4\rangle\langle 1|2+5|6\rangle\langle 5|1+2|4\rangle\langle 5|1+2|6\rangle s_{125}} + \\
& \frac{[12]^6\langle 15\rangle\langle 46\rangle^7(1i\langle 12\rangle[12][23]\langle 34\rangle\langle 45\rangle \dots \langle 6 \text{ terms} \rangle \dots +1i[23]\langle 25\rangle[25]\langle 34\rangle\langle 45\rangle)}{[15]\langle 34\rangle\langle 36\rangle\langle 3|1+5|2\rangle\langle 3|1+2|5\rangle\langle 4|1+5|2\rangle\langle 4|1+2|5\rangle\langle 6|1+5|2\rangle\langle 6|1+2|5\rangle s_{125}} + \\
& \frac{[26]\langle 6|1+2|3\rangle^7(1i\langle 12\rangle[12]\langle 13\rangle[34]\langle 46\rangle \dots \langle 6 \text{ terms} \rangle \dots -1i\langle 16\rangle[24]\langle 26\rangle\langle 34\rangle[36])}{\langle 12\rangle^2\langle 26\rangle[34][35]\langle 45\rangle\langle 1|2+6|3\rangle\langle 1|2+6|4\rangle\langle 1|2+6|5\rangle\langle 6|1+2|4\rangle\langle 6|1+2|5\rangle s_{345}} + \\
& \frac{[12]^6\langle 16\rangle\langle 45\rangle^7(1i\langle 12\rangle[12][23]\langle 34\rangle\langle 46\rangle \dots \langle 6 \text{ terms} \rangle \dots +1i[23]\langle 26\rangle[26]\langle 34\rangle\langle 46\rangle)}{[16]\langle 34\rangle\langle 35\rangle\langle 3|1+6|2\rangle\langle 3|1+2|6\rangle\langle 4|1+6|2\rangle\langle 4|1+2|6\rangle\langle 5|1+6|2\rangle\langle 5|1+2|6\rangle s_{345}} + \\
& \frac{[23]s_{123}^7(1i\langle 12\rangle\langle 13\rangle[14][25]\langle 45\rangle \dots \langle 6 \text{ terms} \rangle \dots -1i\langle 13\rangle[23]\langle 25\rangle\langle 34\rangle\langle 45\rangle)}{\langle 12\rangle^2\langle 23\rangle\langle 45\rangle[46][56]\langle 1|2+3|4\rangle\langle 1|2+3|5\rangle\langle 1|2+3|6\rangle\langle 3|1+2|4\rangle\langle 3|1+2|5\rangle\langle 3|1+2|6\rangle}
\end{aligned}$$
